# Supplementary material for: Sensitivity of MCMC-based analyses to small-data removal
Source: arXiv:2408.07240 source file (2024-11-11)
Supplement: Supplementary file 1 [file appendix_more_experiments.tex]

%

%

%

%
%
%

%
%
%

%
%
%
%
%

%
%
%


%

%
%
%
%

%
%
%
%
%

%

%
%

%
%
%
%
%

%
